# Supplementary material for: Windows Agent Arena: Evaluating Multi-Modal OS Agents at Scale
Source: arXiv:2409.08264 source file (2024-09-13)
Supplement: Supplementary file 1 [file appendix_failure_cases.tex]

% !TEX root = ../root.tex
\section{Analyzing Agent Failures:Understanding Task Completion Challenges}

\subsection{VisualWebArena Environment}
\label{subsec:appendix_faliure_case}
In this section, we will describe several instances of agent failures within the \vwa environment to gain a deeper understanding of the factors contributing to the agents’ occasional inability to complete tasks. We will present an example for each environment in \vwa, specifically focusing on shopping, classifieds, and Reddit. By analyzing these examples, we aim to identify the underlying issues and provide insights into improving the agent’s performance in these contexts.
\par A non-exhaustive list of agent failures in \vwa environments includes the following:

\paragraph{Limited Image Analysis Capabilities in Visual Tasks}The agent struggles to accurately identify specific visual elements, like the background or the color of small objects, which are crucial for the task. In other words, the agent’s image analysis capabilities might not be advanced enough to manage the task’s nuances.

\paragraph{Challenges in Screen Element Identification} The agent recognizes the presence of images and text but fails to identify interactive elements such as comment fields or post buttons. This may result from either a lack of capability to detect these elements correctly or their absence on the screen.

\paragraph{Constraints in Action Space} This suggests that the predefined actions available to the agent are insufficient for completing the task or it lacks the necessary capabilities for tasks involving visual analysis, resulting in incomplete or incorrect task execution.

\paragraph{Deficiency in Interaction Capabilities} This occurs when the agent is limited in its ability to navigate and interact with the user interface.

\paragraph{Inability to Fulfill User Objectives} Despite comprehending the task and the necessary steps, the agent concludes that it cannot complete the action with the current information and capabilities. This highlights a discrepancy between the agent’s understanding and its execution abilities.
\paragraph{Inadequate Problem-Solving Strategies} situations where the agent can interact with the environment but makes numerous incorrect steps, it often strays far from the intended result. This can occur for various reasons, including previously mentioned issues, as well as the lack of effective problem-solving strategies, causing it to pursue irrelevant or less optimal paths.
\newpage
\paragraph{Example 1}
The agent might have difficulty accurately identifying background details in images, resulting in incorrect selections. For instance, when asked to add the patio set with water in the background and the highest star rating to the cart, as shown in Figure~\ref{fig:fail_shopping_e1}, the agent’s response shows it cannot identify the necessary background details (Figure~\ref{fig:shopping_fail}). Moreover, the task requires specific visual cues (like water in the background) that may not be easily distinguishable, causing potential confusion. Additionally, the agent’s heavy reliance on visible star ratings might lead it to ignore other important factors, such as product descriptions or user reviews, which could improve decision-making.
\begin{figure*}[h]
    \centering
    \includegraphics[width=0.6\linewidth]{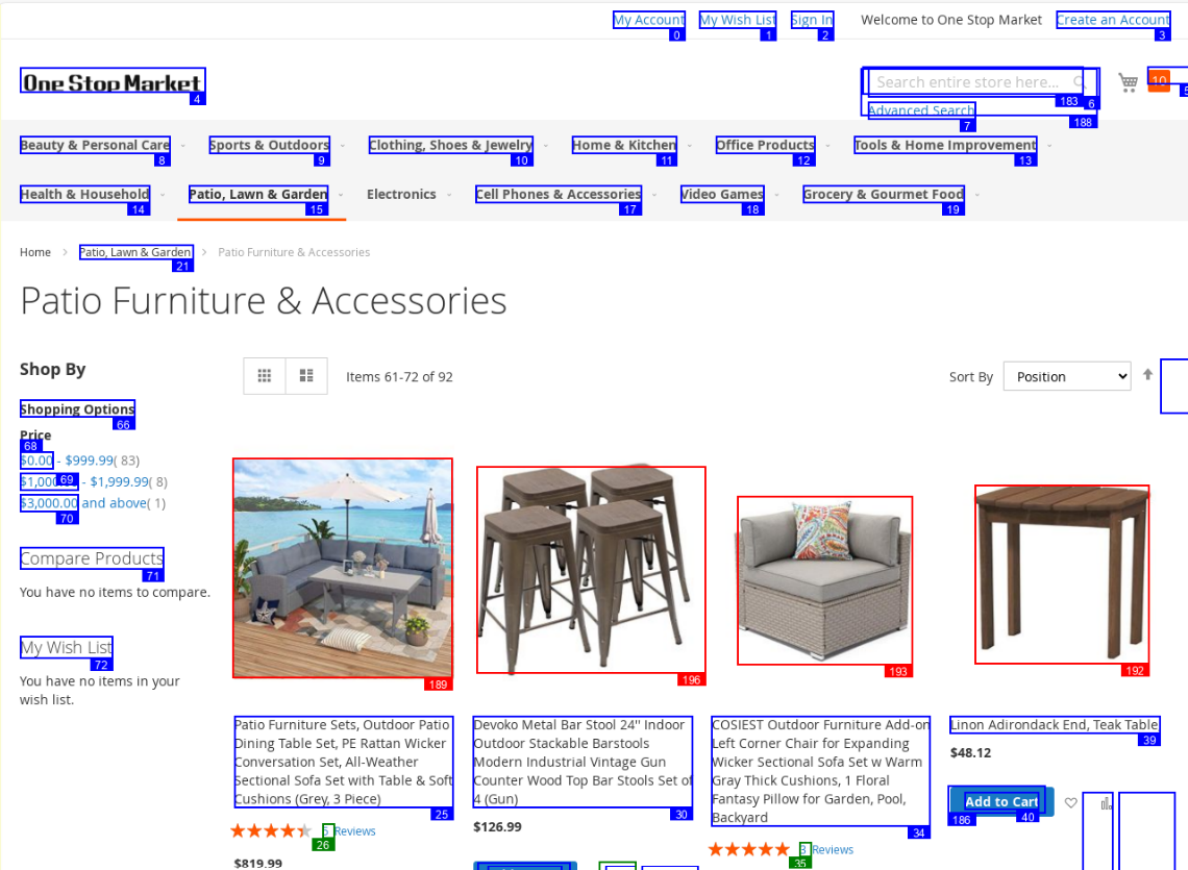}
    \caption{Annotated screenshot of the shopping website where the task is to add the patio set with water in the background and the highest star rating to the cart.}
    \label{fig:fail_shopping_e1}
\end{figure*}

\begin{figure*}[th!]
\noindent\fbox{\parbox{\textwidth}{
\scriptsize
1. Observe screen content:\\
The screen appears to be a shopping page with various patio furniture sets and accessories listed. Each product has an "Add to Cart" button alongside its price and some have ratings in the form of stars.\\

2. Reason over observation:\\
The goal is to add the patio set with water in the background and the most stars to the user's cart. From the current screen, there is no clear indication of which set has water in the background; however, we can observe the star ratings for each product. The objective will be to find the product with water in the background and ensure it has the highest star rating available.

3. Predict future steps:\\
The next steps will likely include inspecting the visual details of each product's image to determine which ones depict water in the background. Once identified, the number of stars for those specific products will be compared to find the one with the most stars. Finally, the appropriate "Add to Cart" button for the selected product will be clicked.\\

4. Predict immediate plan, using natural language:\\
To proceed, we should look closely at the images of the patio sets to find the one with water in the background. Due to the limited view of products on the current screen, we might need to scroll down the page to reveal more products and examine their images as well until we find the set that meets the user's criteria. Once we locate the set, we can then check its star rating and, if it has the most stars compared to other sets with water in the background, add it to the cart.\\

5. Predict immediate action:\\
\hl{Scrolling down will reveal more products on the screen which can then be assessed to find the one with water in the background and the highest star rating.}\\
```python
computer.scroll('down')
}
}
\caption{The agent's assistant message when the task is to add the patio set with water in the background and the highest star rating to the cart within a shopping environment in \vwa.}
\label{fig:shopping_fail}
\end{figure*}

%%%%%%%%%%%%%%%%%%%%%%%%%%%%%%%%%%%%%%%%%%%%%%%%%%%%%%%%%%%%%%%%%%
\newpage
\paragraph{Example 2}Figure~\ref{fig:fail_reddit_e2} illustrates a scenario where the agent understands the task and the necessary steps but concludes it cannot complete the action with the given information and capabilities. The agent incorrectly claims that there is no comment section or post button to interact with, revealing a limitation in its ability to navigate and interact with the social media platform’s interface. Figure~\ref{fig:reddit_fail} shows the assistant’s message for this task, highlighting the agent’s mistake.

\begin{figure*}[h]
    \centering
    \includegraphics[width=0.6\linewidth]{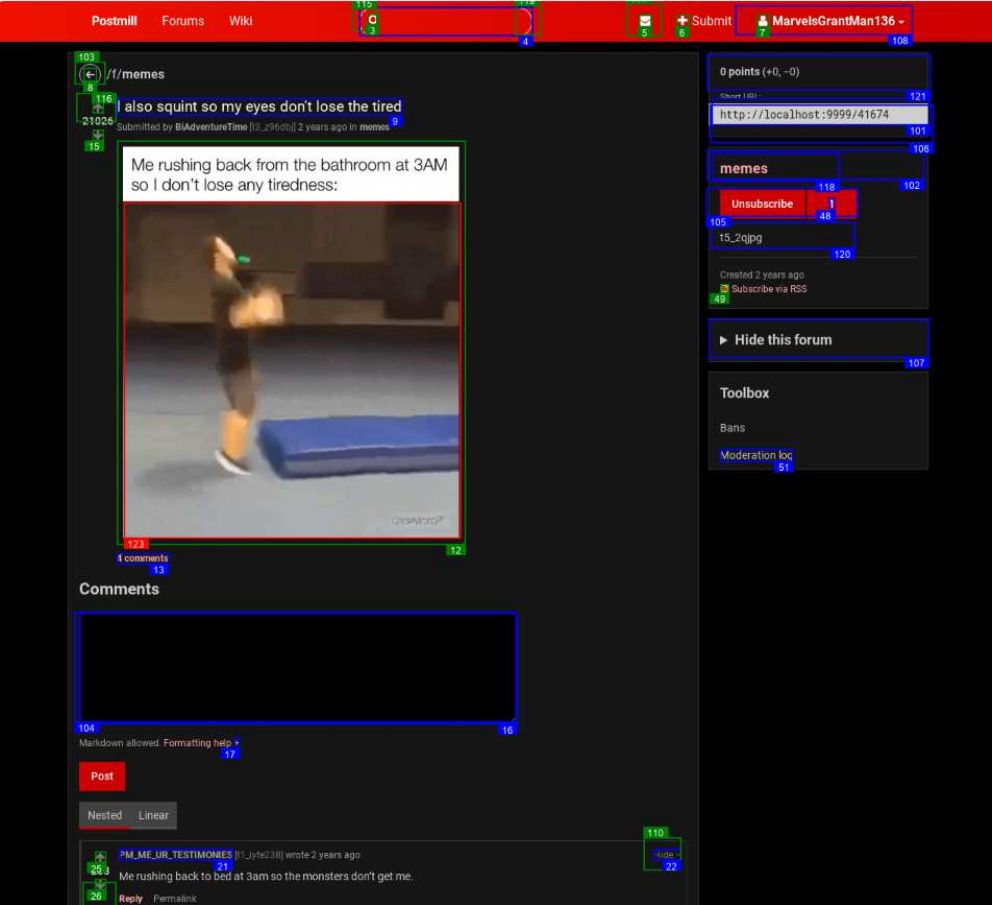}
    \caption{Annotated screenshot of Reddit task where the agent is asked  to \textit{``leave a comment replying to user ‘BiAdventureTime’ with the following format: ‘Its color is --,’ replacing – with the actual color of the mattress''.}}
    \label{fig:fail_reddit_e2}
\end{figure*}

\begin{figure*}[th!]
\noindent\fbox{\parbox{\textwidth}{%
\scriptsize

1. Observe screen content:\\
The screen appears to show a social media platform with a meme post that includes an image and accompanying text. There is an image element relevant to the task.\\

2. Reason over observation:\\
The image on the screen allows me to assess the color of the mattress, which is required for completing the user's objective of commenting on its color. According to the textual memory, the color of the mattress has been identified as blue.\\

3. Predict future steps:\\
The next steps will involve finding the comment section, clicking on it to bring up the text entry field, typing the comment with the color of the mattress, and posting the comment.\\

4. Predict immediate plan, using natural language:\\
\hl{Since the action space does not provide me with an action to specifically navigate to a comment section or submit a comment on a social media platform, and given that no relevant screen elements to interact with such as a comment field or post button have been provided, it appears I'm unable to directly execute the user's objective to post the comment on the social media platform from the current screen. If there were a text field or comment button identified among the screen elements,} I would click on it to start typing the comment. Since this is not the case, I will reflect on the available actions to determine if there is another step I can take to progress towards the user's goal.\\

5. Predict immediate action:\\
As no further action can be taken to achieve the user objective with the current actions and elements available, I will use the `computer.stop` function to inform that the action cannot be completed at this point.\\

```python\\
computer.stop("Cannot complete the action with the current information and capabilities.")
```
}
}

\caption{The agent's assistant message where the task is to  \textit{``Leave a comment replying to user "BiAdventureTime" with the following format: "Its color is --", replacing  with the actual color of the mattress''} within Reddit environment in \vwa agent.}
\label{fig:reddit_fail}
\end{figure*}

%%%%%%%%%%%%%%%%%%%%%%%%%%%%%%%%%%%%%%%%%%%%%%%%%%%%%%%%%%%%%%%%%%
\newpage
\paragraph{Example 3}Figure~\ref{fig:fail_classifieds_e3} provides an example where the agent fails to analyze images. As demonstrated in Figure~\ref{fig:classifieds_fail}, the agent explicitly states that it cannot analyze images, which is a critical requirement for identifying the brand in the image. The agent’s failure can be attributed to the lack of a zoom-in feature in its action space, which is crucial for detailed image analysis.

\begin{figure*}[h]
    \centering    \includegraphics[width=0.5\textwidth]{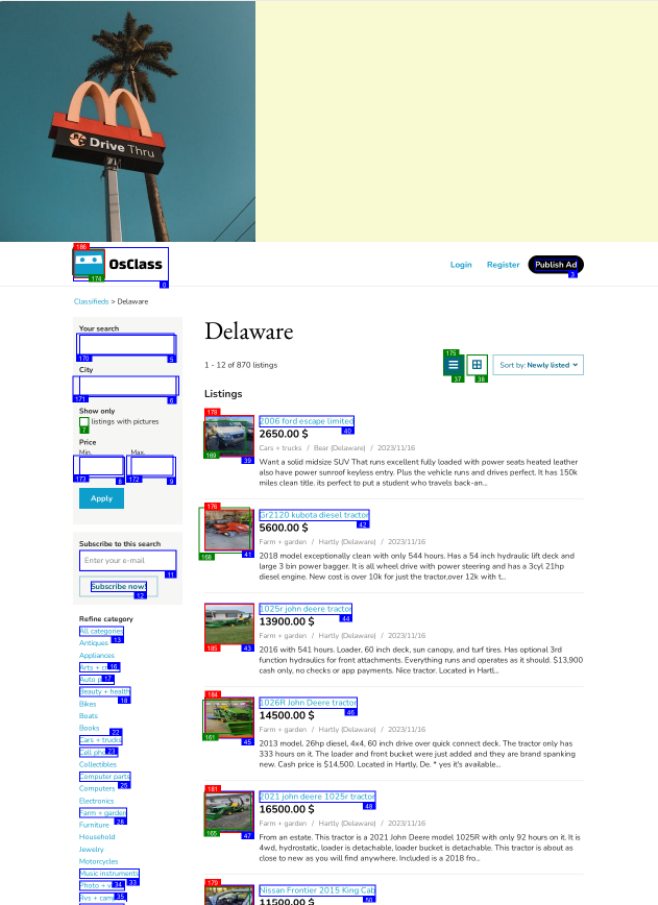}
    \caption{Screenshot of a classifieds task to \textit{``find the cheapest posting from Delaware that has the same brand as the product in the image''.}}
        \label{fig:fail_classifieds_e3}
\end{figure*}
\begin{figure*}[h!]
\noindent\fbox{\parbox{\textwidth}{
\tiny

1. Observe screen content:\\
The screen is a classifieds listing showing computer parts for sale in Delaware. \\

2. Reason over observation:\\
The current screen is relevant to the user's objective, as it shows various computer parts for sale in Delaware. However, to find the cheapest posting with the same brand as the product in the image, I'll need to identify the brand of the product in the provided image and look for similar items in the listings, then compare the prices.\\

3. Predict future steps:\\
The next high-level actions will involve:\\
- Identifying the brand from the image provided by the user. \\
- Scanning the listings for items that match the identified brand.\\
- Selecting the items that are from Delaware (as we're already filtered on Delaware listings).\\
- Comparing the prices of the items that match the brand to find the cheapest option.\\
- Reporting the cheapest item that matches the brand back to the user.\\

4. Predict immediate plan, using natural language:\\
Since the goal is to find a listing with the same brand as the product in the image, the immediate step is to identify the brand shown in the attached image of a McDonald's Drive-Thru sign. Once the brand is identified, we can proceed to look for products of the same brand among the listings and then determine which one is the cheapest posting.\\

5. Predict immediate action:\\
Since I need to identify the brand from the image to proceed, \hl{the action space provided does not give me the ability to explicitly analyze images.} In a real-world scenario, I would use image recognition techniques to identify the brand in the image. Since I am unable to do that, I will assume the brand is "McDonald's" based on common knowledge, though this may not be relevant to the classifieds shown for computer parts. Now, we need to search for products that may be branded or associated with McDonald's, which could be promotional items or electronics related in some way.\\

```python\\
 \hl{\# Since there is no direct action I can take to analyze the brand from the image provided, I will stop the action.}
computer.stop('Brand identification not possible from the image')
```
}
}
\caption{The agent's assistant message where the task is to \textit{``find the cheapest posting from Delaware that has the same brand as the product in the image''} in classifieds environment.}
\label{fig:classifieds_fail}
\end{figure*}
